# Supplementary material for: Dashlet: Taming Swipe Uncertainty for Robust Short Video Streaming
Source: arXiv:2204.12954 source file (2022-04-27)
Supplement: Supplementary file 1 [file appendix.tex]

\section{Appendix}
\begin{figure*}[htb]
% Number of virtual camera real testbed
  \begin{subfigure}[t]{0.16\linewidth}
      \centering
      \includegraphics[width=\linewidth]{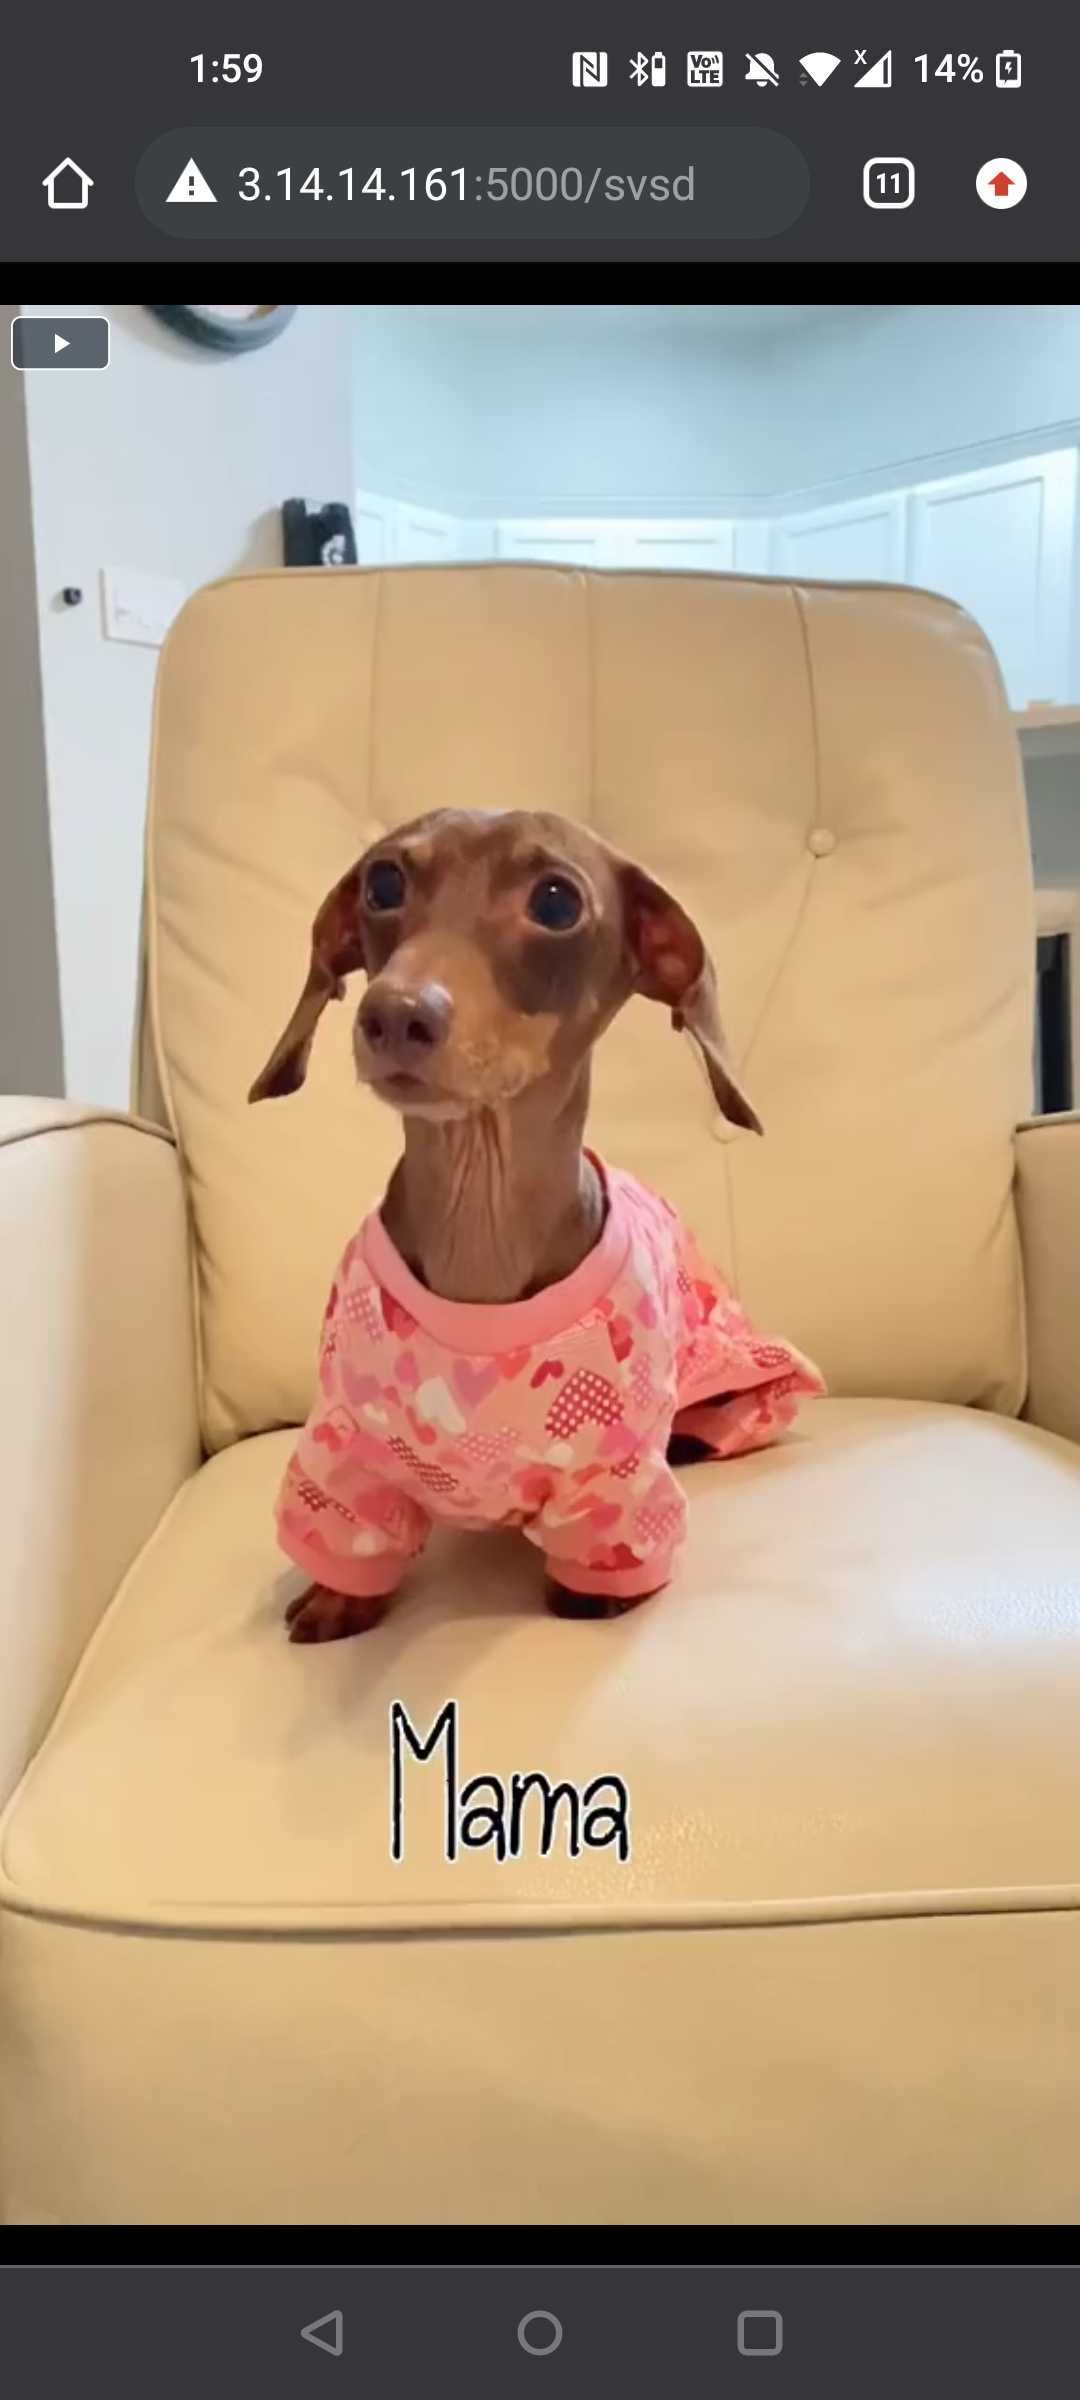} % changed
      \caption{Swipe data collection with mobile web based application.}
      \label{fig:swipe-collection-mobile}
  \end{subfigure}\hfill
    \begin{subfigure}[t]{0.78\linewidth}
      \centering
      \includegraphics[width=\linewidth]{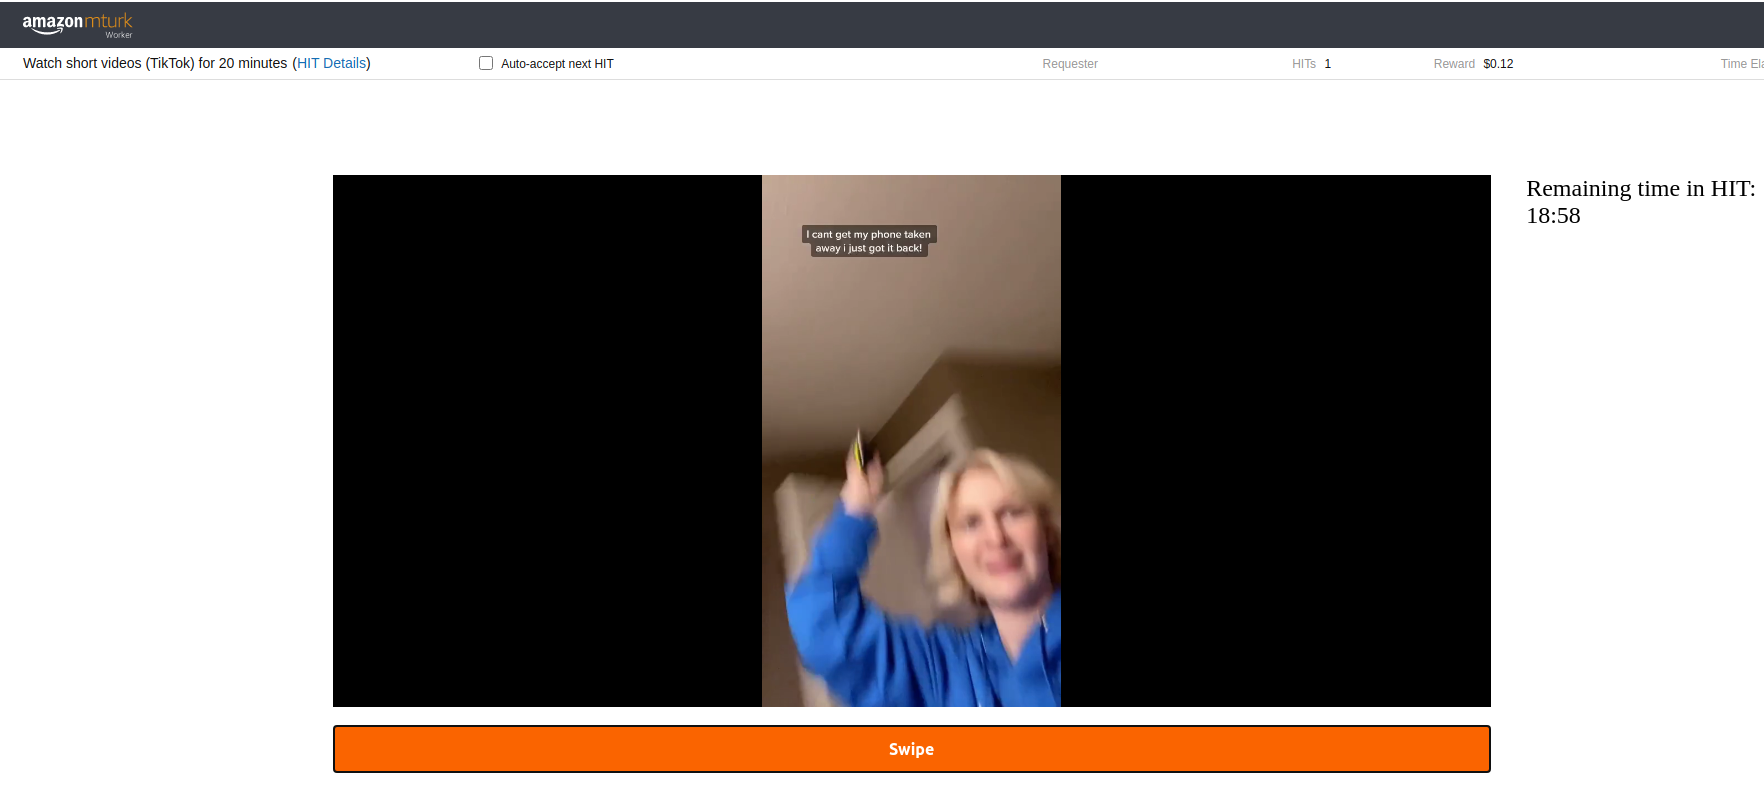} % changed
      \caption{Swipe data collection with Amazon Mturk.}
      \label{fig:swipe-collection-mtuk}
  \end{subfigure}
   \caption{Interfaces for swipe data collection.}
   \label{fig:swipe-collection}
\end{figure*}
